# Supplementary material for: RCL: Recurrent Continuous Localization for Temporal Action Detection
Source: arXiv:2203.07112 source file (2022-03-14)
Supplement: Supplementary file 1 [file tal.pdf]

# Supplementary Material for
# RCL: Recurrent Continuous Localization for Temporal Action Detection

Anonymous CVPR submission

Paper ID 549

**Appendix**

In this supplementary material, we provide additional implementation details for our method (Section 1) and show additional qualitative results (Section 2).

## 1. Implementation Details

In this section, we present some implementation details that were omitted in the main paper for brevity.

The RCL module is general, and can be applied to other action detection frameworks [4,7]. BMN [4] is a grid-based detector which utilizes the boundary-matching network to improve the efficienc for retrieving proposals [5]. Our RCL module can be directly applied to replace the proposal evaluation module (as Figure 1). G-TAD [7] is a state-of-the-art action detector which employs a well-designed graph module, GCNeX, to improve the temporal representation. Since there is no special optimization objects for the architecture, we use the improved feature in our RCL framework. Other settings are maintained the same as those for BMN.

### 1.1. General components for our baseline

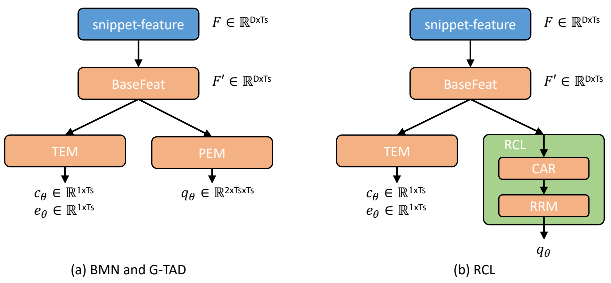


Figure 1. Design of applying RCL to BMN and G-TAD, illustrated with abstractions.

Although the model architectures of different detectors [4, 7] are different, they have common components, which can be roughly summarized into the following classes:

**Base Feature** is the part that enhances the original snippet features with more context. BMN adopts stacks of local convolutions to capture local-range context. G-TAD utilize structured graphs to model long-range dependencies.

**TEM** is the part that predicts the starting and ending probabilities for all temporal locations. BMN use these boundary probability to generate more reliable confidence scores. G-TAD and our RCL utilize this module to regularize the training process.

**PEM** is the part that predicts tIoU and classification scores on dense locations of feature maps. Specifically, BMN use Boundary-Matching Layer [4] to sample all segment features, and G-TAD utilizes SGAlign [7] to extract sub-graph features.

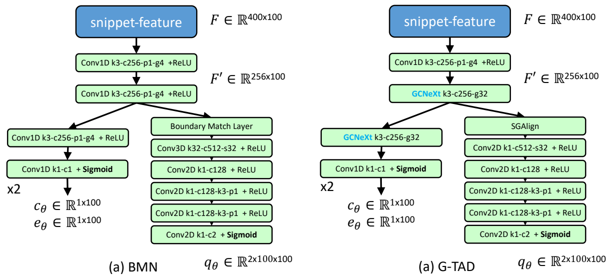


Figure 2. The feed-forward network for BMN and G-TAD.

By forwarding the snippet features into a convolutional network (see Figure 2), the proposal confident scores are computed which can be represented to the $2 \times D \times T_s$ feature maps. For THUMOS14 [3] and ActivityNet v1.3 [2], we set $D = 64, T_s = 256$ for THUMOS14 and $D = 100, T_s = 100$ for ActivityNet v1.3 for both baseline [4, 7].

**Feature alignment for CAR.** As shown in Figure 3, we use the nearest regular grid feature as the temporal representation and add two additional input channel for temporal coordinates. We achieve *continuity* by densely sampling coordinates. For the regular grid feature, we sample 32 points and extend the boundary region with 0.5 segment length, following the original implementations [4].

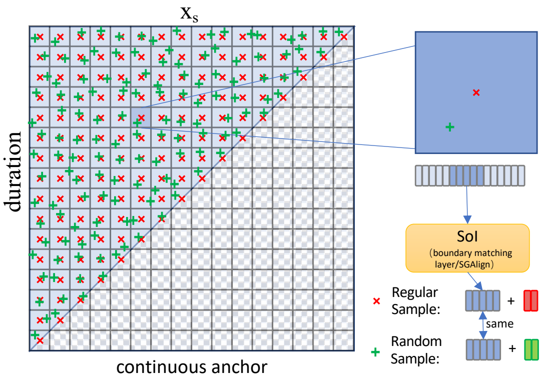


Figure 3. The feature alignment for continuous representation.

```
def forward(self, base_feat, heatmap, iters=10, hdim=64, cdim=32):
    heatmap = torch.logit(heatmap)  # inverse sigmoid
    base_feat = base_feat.contiguous()

    # run the context network
    with autocast(enabled=self.mixed_precision):
        cnet = self.cnet(base_feat)
        net, inp = torch.split(cnet, [hdim, cdim], dim=1)
        net = torch.tanh(net)
        inp = torch.relu(inp)

    heatmap_predictions = []
    for itr in range(iters):
        heatmap = heatmap.detach()
        with autocast(enabled=self.mixed_precision):
            net, up_mask, delta_heatmap = self.update_block(
            net, inp, base_feat, heatmap)

        heatmap = heatmap + delta_heatmap
    return heatmap
```

Figure 4. Python code of RRM based on PyTorch.

**Network for RRM.** Inspired by the recent success in Recurrent All-Pairs Field Transforms for Optical Flow (RAFT [6]), we utilize the `SmallUpdateBlock` to refine the confidence maps. The update operator is a gated activation unit based on the variant of GRU cell:

$$
\begin{aligned}
z_t &= \sigma\left(\mathrm{Conv}_{3\times3}\left(\left[h_{t-1}, x_t\right], W_z\right)\right) \\
r_t &= \sigma\left(\mathrm{Conv}_{3\times3}\left(\left[h_{t-1}, x_t\right], W_r\right)\right) \\
\tilde{h}_t &= \tanh\left(\mathrm{Conv}_{3\times3}\left(\left[r_t \odot h_{t-1}, x_t\right], W_h\right)\right) \\
h_t &= \left(1 - z_t\right) \odot h_{t-1} + z_t \odot \tilde{h}_t
\end{aligned} \tag{1}
$$

where $x_t$ is the concatenation of confidence scores $\mathbf{G}_t$, temporal features, and context features. The main forward code are shown in Figure 4.

## 2. Additional Results

**Scale imbalance:** In Figure 5 we show the sensitivity average-mAP$_N$ analysis, generated by the DETAD toolbox [1], for BMN baseline with different sample densities.

First, we compared three sampling methods: (1) regular grid sampling, (2) reducing the sample ratio of $0.5\times$ for region with the duration greater than 0.5. (3) reducing the

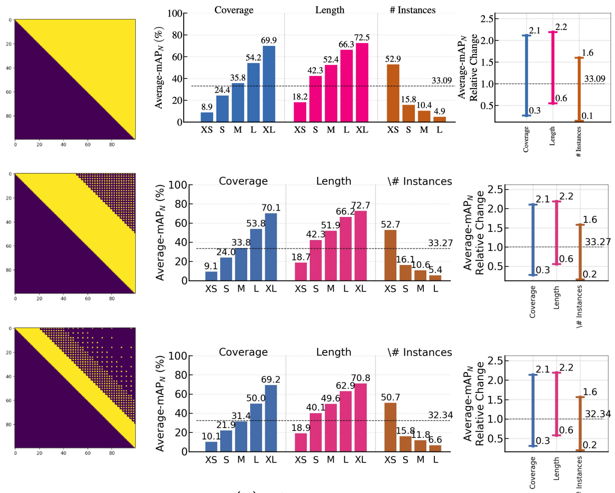


(a) sparse sample (b) The sensitivity average-mAP$_N$.

Figure 5. The effect for irregular sample strategy. A large number of redundant proposals exist for long-term segments.

| Iter Steps | Feature | AP@0.5 | mAP | Flops |
|---|---|---|---|---|
| 0 | TSN | 52.35 | 35.41 | **98.3** |
| 1 | TSN | 52.24 | 35.60 | 100.0 |
| 5 | TSN | 53.62 | 35.85 | 106.9 |
| 10 | TSN | **54.19** **(+1.84)** | **35.98** **(+0.57)** | 115.5 |
| 15 | TSN | 53.98 | 35.64 | 124.1 |

Table 1. Ablation experiments on ActivityNet v1.3 for iterations.

sample ratio of $0.5^l\times$ for region with the duration parameter $l = \lfloor duration/0.2 \rfloor$. These sparse sample strategy are proposed in 2D-TAN [8]. By reducing the sampling density for the long-term segment, we can see that the overall performance has not dropped too much and the mAP$_N$ for Coverage-XS is improve.

Note that while the sparse sampling method uses fewer anchors, the amount of calculation remains the same as the regular one. The discretized grid structure inherently limits the flexibility of dynamic sampling. To maximally excavate redundancy in the grid representation, our RCL can dynamically instantiate any segments. Compared with regular grid sample strategy and the sparse sample strategy, our continuous representation and scale-invariant sample strategy has a great advantage in predicting short-term and also performs better for long segments.

**Iterative steps for RRM:** As shown in Table 1, our recurrent refine module (RRM) achieves the best results in 10 iterations, which only adds 17% FLOPs. Our proposed model obtains a good trade-off between accuracy and computational cost. More iterations usually improve mAP and improvements saturate at 10 steps, which may be related to overfitting.

# References


[1] Humam Alwassel, Fabian Caba Heilbron, Victor Escorcia, and Bernard Ghanem. Diagnosing error in temporal action detectors. In *Proceedings of the European Conference on Computer Vision (ECCV)*, pages 256–272, 2018. 2

[2] Fabian Caba Heilbron, Victor Escorcia, Bernard Ghanem, and Juan Carlos Niebles. Activitynet: A large-scale video benchmark for human activity understanding. In *Proceedings of the ieee conference on computer vision and pattern recognition*, pages 961–970, 2015. 1

[3] Y.-G. Jiang, J. Liu, A. Roshan Zamir, G. Toderici, I. Laptev, M. Shah, and R. Sukthankar. THUMOS challenge: Action recognition with a large number of classes. http://crcv.ucf.edu/THUMOS14/, 2014. 1

[4] Tianwei Lin, Xiao Liu, Xin Li, Errui Ding, and Shilei Wen. Bmn: Boundary-matching network for temporal action proposal generation. In *Proceedings of the IEEE/CVF International Conference on Computer Vision*, pages 3889–3898, 2019. 1

[5] Tianwei Lin, Xu Zhao, Haisheng Su, Chongjing Wang, and Ming Yang. Bsn: Boundary sensitive network for temporal action proposal generation. In *Proceedings of the European Conference on Computer Vision (ECCV)*, September 2018. 1

[6] Zachary Teed and Jia Deng. Raft: Recurrent all-pairs field transforms for optical flow. In *European conference on computer vision*, pages 402–419. Springer, 2020. 2

[7] Mengmeng Xu, Chen Zhao, David S Rojas, Ali Thabet, and Bernard Ghanem. G-tad: Sub-graph localization for temporal action detection. In *Proceedings of the IEEE/CVF Conference on Computer Vision and Pattern Recognition*, pages 10156–10165, 2020. 1

[8] Songyang Zhang, Houwen Peng, Jianlong Fu, and Jiebo Luo. Learning 2d temporal adjacent networks for moment localization with natural language. In *Proceedings of the AAAI Conference on Artificial Intelligence*, volume 34, pages 12870–12877, 2020. 2
